# Supplementary material for: Distillation Learning Guided by Image Reconstruction for One-Shot Medical Image Segmentation
Source: arXiv:2408.03616 source file (2025-01-05)
Supplement: Supplementary file 1 [file appendix.tex]

% \newpage

% %\onecolumn
% \section*{Appendix}
% This document serves as an appendix to our research, "Distillation Learning Guided by Image Reconstruction for One-Shot Medical Image Segmentation". We provide additional technical details on the bilinear interpolation-based image-to-image warping operation, along with visualizations of the intermediate synthetic images and labels generated by the teacher network for the OASIS, BCV, and VerSe datasets. Furthermore, we include additional experimental results and their analysis. To ensure reproducibility, a detailed description of the experimental settings mentioned in the main paper is provided. Additionally, access to our trained model, code, and demonstration examples is available through an anonymized link: https://github.com/NoviceFodder/OS-MedSeg.

% \subsection{Details of Spatial Transformer Networks}
% \label{details-stl}
% The proposed method aims to optimize parameter values by minimizing dissimilarities between the fixed, unlabeled image $y$ and the warped image $x \circ \phi$. To enable the application of standard gradient-based techniques, we introduce a differentiable operation that leverages spatial transformer networks \cite{jaderberg2015spatial} for computing $x \circ \phi$.

% For every voxel $\mathbf{p}$, we compute a (subpixel) voxel location $\mathrm{p' = p + u(p)}$ in $y$. Since image values are defined only at integer locations, we employ linear interpolation to determine values from the eight neighboring voxels:

% \begin{equation}
% x\circ\phi(\mathbf{p})=\sum_{\mathbf{q}\in\mathcal{Z}(\mathbf{p}^{\prime})}x(\mathbf{q})\prod_{d\in\{x,y,z\}}(1-|\mathbf{p}_d^{\prime}-\mathbf{q}_d|),
% \end{equation}

% where $\mathcal{Z}(\mathbf{p}^{\prime})$ represents the voxel neighbors of $\mathbf{p}^{\prime}$, and $d$ iterates over the dimensions of $\Omega$.
% \subsection{Additional Experimental Results}
% In this section, we present additional visualizations of our experiments. 

% \textcolor[rgb]{0.0, 0.56, 0.8}{Fig.} \ref{fig:recon-syn} displays images generated during the intermediate stages of our framework, including synthetic images and their corresponding synthetic labels produced by the synthesis network, as well as reconstructed images generated by the teacher network. We showcase visual results on three datasets: OASIS, BCV, and VerSe.

% \textcolor[rgb]{0.0, 0.56, 0.8}{Fig.} \ref{fig:OASIS_boxplots} presents DSC across different brain tissues for both state-of-the-art methods and our method's segmentation results on all test images within the OASIS dataset.

% \textcolor[rgb]{0.0, 0.56, 0.8}{Table} \ref{tab:bcv_detail} presents DSC across different abdominal organs for both state-of-the-art methods and our method's segmentation results on all test images within the BCV dataset.


% \begin{figure}[ht]
%     \centering
%     \includegraphics[width=0.5\textwidth]{LaTeX/figures/recon_syn.png}
%     \caption{The visualization includes the initial unlabeled image, the synthetic image, the synthetic label, and the reconstructive image. Example 2D slices of
%     randomly selected cases from the OASIS, BCV, and VerSe datasets are displayed from top to bottom. Notably, the synthetic images and labels are paired, generated from the image synthesis network. The reconstructive images are generated from the teacher network.
% }
%     \label{fig:recon-syn}
% \end{figure}

% \begin{table}[th]
% \scriptsize
% \setlength{\tabcolsep}{3pt}
% \renewcommand{\arraystretch}{1.0}
% \caption{Quantitative evaluation results of the segmentation of four abdomen organs on the BCV dataset. Fully supervised segmentation was used as the benchmark for the upper performance limits. Dice Similarity Coefficient (DSC) for various abdomen organs were calculated, with means and standard deviations reported. The best result, excluding the upper limit, is highlighted in \textbf{\textcolor[rgb]{0.0, 0.56, 0.8}{blue}}.}
% \label{tab:bcv_detail}
% \centering
% \begin{tabular}{lcccccc}
%     \toprule
%     \multirow{2}{*}{\textbf{Method}} & \multirow{2}{*}{\textbf{Type}} & \multicolumn{5}{c}{\textbf{DSC $\uparrow$}} \\ 
%     \cmidrule(lr){3-7}
%     & & \textbf{Liver} & \textbf{Spleen} & \textbf{R-Kidney} & \textbf{L-Kidney} & \textbf{Mean $\pm$ Std} \\
%     \midrule
%     Supervised \cite{he2016deep} & LS & \textbf{0.960} & \textbf{0.940} & \textbf{0.873} & \textbf{0.864} & \textbf{0.919 $\pm$ 0.056} \\  
%     \midrule
%     U-Net \cite{ronneberger2015u}& LS & 0.863 & 0.339 & 0.407 & 0.413 & 0.538 $\pm$ 0.110 \\  
%     ResUNet\cite{he2016deep} & LS & 0.867 & 0.634 & 0.417 & 0.421 & 0.609 $\pm$ 0.148 \\  
%     \midrule
%     Affine\cite{arun1987least} & Trad & 0.768 & 0.437 & 0.496 & 0.520 & 0.561 $\pm$ 0.101 \\ 
%     SyN\cite{avants2008symmetric} & Trad & 0.860 & 0.733 & 0.698 & 0.748 & 0.768 $\pm$ 0.108 \\ 
%     \midrule
%     VoxelMorph-1\cite{balakrishnan2018unsupervised} & ABS & 0.841 & 0.732 & 0.625 & 0.572 & 0.700 $\pm$ 0.097 \\ 
%     VoxelMorph-2 \cite{balakrishnan2019voxelmorph}& ABS & 0.847 & 0.747 & 0.647 & 0.633 & 0.726 $\pm$ 0.103 \\ 
%     TransMorph\cite{chen2022transmorph} & ABS & 0.854 & 0.781 & 0.703 & 0.694 & 0.766 $\pm$ 0.103 \\ 
%     CLMorph\cite{liu2023contrastive} & ABS & 0.845 & 0.756 & 0.650 & 0.625 & 0.726 $\pm$ 0.108 \\     
%     \midrule
%     DataAug\cite{zhao2019data} & LRLS & \textbf{\textcolor[rgb]{0.0, 0.56, 0.8}{0.914}} & 0.854 & 0.756 & 0.734 & 0.822 $\pm$ 0.103 \\ 
%     BRBS\cite{he2022learning} & LRLS & 0.892 & 0.711 & 0.784 & \textbf{\textcolor[rgb]{0.0, 0.56, 0.8}{0.804}} & 0.806 $\pm$ 0.113 \\ 
%     \midrule
%     DR-OMSeg & LRLS & 0.903 & \textbf{\textcolor[rgb]{0.0, 0.56, 0.8}{0.863}} & \textbf{\textcolor[rgb]{0.0, 0.56, 0.8}{0.799}} & 0.729 & \textbf{\textcolor[rgb]{0.0, 0.56, 0.8}{0.846 $\pm$ 0.084}} \\ 
%     \bottomrule
% \end{tabular}
% \end{table}

% \begin{figure*}[ht]
%     \centering
%     \includegraphics[width=1.0\textwidth]{LaTeX/figures/OASIS_boxplots.png}
%     \caption{Boxplots of Dice scores across various anatomical structures for segmentation results on all test images in the OASIS dataset. For the purpose of this visualization, we aggregate DSC of the left and right brain hemispheres into a single score. We use abbreviated labels: white matter (WM), cortex (CX) and ventricle (vent).}
%     \label{fig:OASIS_boxplots}
% \end{figure*}
